# Supplementary material for: StoryVerse: Towards Co-authoring Dynamic Plot with LLM-based Character Simulation via Narrative Planning
Source: arXiv:2405.13042 source file (2024-11-02)
Supplement: Supplementary file 1 [file appendix.tex]

\begin{small}
\begin{algorithm}
\caption{LLM-based Narrative Planning}
\label{alg:narrative_planning}
\KwIn{$G$: narrative goal as a natural language statement; $W$: world state; $\mathcal{D}$: story domain; $maxStep$: maximum number of revisions}
\KwOut{A sequence of character actions}
$plan$ $\leftarrow$ \parbox[t]{.6\linewidth}{%
$PlanGenerator.GeneratePlan$($G$, $W$, $\mathcal{D}$, {\it feedback = null});}

\bf{while} $plan$ is not executable and $maxStep$ not reached:
\begin{enumerate}
    \item $feedback_{overall}$ $\leftarrow LLM.PlotCoherencyQuery(plan)$    \item $feedback_{game}$ $\leftarrow \emptyset$;
    \item $feedback_{ch}$ $\leftarrow \emptyset$;
    \item \bf{for each} $action\in plan$ (in order):
        \begin{enumerate}
            \item $feedback_{game}$ $+=$ $GameEnv.Execute$($action$);
            \item $feedback_{ch}$ $+=$ $LLM.CharacterMotivationQuery$($action$); 
            \item if $LLM.NarrativeGoalMetQuery$($plan_{action}$, $G$):\\
            \ \ \ \ return $plan_{action}$;
    \item $f$ $\leftarrow$  $feedback_{overall}$ + $  feedback_{game}$ + $feedback_{ch}$;
    \item $plan$ $\leftarrow$ \parbox[t]{.6\linewidth}{%
$PlanGenerator$.$GeneratePlan$($G$, $W$, $\mathcal{D}$, {\it feedback} = $f$);}
        \end{enumerate}
\end{enumerate}
\end{algorithm}
\end{small}

\section{Raw output of "A kindness is never wasted" on Ant \& Dove world}

\begin{lstlisting}
------------------------------
Daily Life
------------------------------
{
    "action": "moveTo(bank)",
    "thought": "I should head to the bank to find some food and maybe meet other creatures. It's always nice to socialize and share the latest news.",
    "subject": "ant"
}
{
    "action": "moveTo(bank)",
    "thought": "I feel like visiting the bank today. It's always nice to meet new friends and maybe I'll see the ant there.",
    "subject": "dove"
}
{
    "action": "moveTo(bank)",
    "thought": "I should head to the bank. It's a good spot to find targets, and I might encounter some animals there. Plus, being close to water could provide additional opportunities.",
    "subject": "hunter"
}
------------------------------
Act : Some character got in an accident and their life is in danger.
(Some character got in an accident and their life is in danger.)
------------------------------
initial plan:
[
        {
                "subject": "ant",
                "action": "moveTo(brook)",
                "thought": "I see some delicious looking leaves across the brook. I should go there to eat."
        },
        {
                "subject": "ant",
                "action": "slipIntoWater()",
                "thought": "Oh no, the edge is slippery! I'm falling into the water!"
        },
        {
                "subject": "dove",
                "action": "moveTo(brook)",
                "thought": "I see the ant in trouble in the water. I need to help!"
        },
        {
                "subject": "dove",
                "action": "save(ant)",
                "thought": "I'll drop a leaf for the ant to climb on and get back to safety."
        },
        {
                "subject": "hunter",
                "action": "tryToKill(dove)",
                "thought": "While the dove is distracted saving the ant, it's a perfect opportunity for me to hunt."
        },
        {
                "subject": "dove",
                "action": "moveTo(oak_tree)",
                "thought": "I sense danger! I must fly away quickly to avoid the hunter."
        },
        {
                "subject": "hunter",
                "action": "think(\"The dove escaped. I should be more careful next time.\")",
                "thought": "The dove escaped. I should be more careful next time."
        }
]
------- revision round 0------

feedback: - hunter tryToKill(dove) is not executable because hunter is not at the same location as dove. hunter should move to brook before taking this action.

- The event hunter.think("The dove escaped. I should be more careful next time.") does not make sense: It does not make sense for the hunter to think 'The dove escaped. I should be more careful next time.' based on the provided current state. There is no information or event mentioned about the hunter attempting to catch the dove or the dove escaping from the hunter. The hunter's motivation and actions have been towards finding a target in general, not specifically targeting the dove.

revised plan: [
        {
                "subject": "ant",
                "action": "moveTo(brook)",
                "thought": "I see some delicious looking leaves across the brook. I should go there to eat."
        },
        {
                "subject": "ant",
                "action": "slipIntoWater()",
                "thought": "Oh no, the edge is slippery! I'm falling into the water!"
        },
        {
                "subject": "dove",
                "action": "moveTo(brook)",
                "thought": "I see the ant in trouble in the water. I need to help!"
        },
        {
                "subject": "dove",
                "action": "save(ant)",
                "thought": "I'll drop a leaf for the ant to climb on and get back to safety."
        },
        {
                "subject": "hunter",
                "action": "moveTo(brook)",
                "thought": "I see a dove distracted by trying to save an ant. This is my chance."
        },
        {
                "subject": "hunter",
                "action": "tryToKill(dove)",
                "thought": "While the dove is distracted saving the ant, it's a perfect opportunity for me to hunt."
        },
        {
                "subject": "dove",
                "action": "moveTo(oak_tree)",
                "thought": "I sense danger! I must fly away quickly to avoid the hunter."
        }
]
The following plot has been generated:
[
    {
        "subject": "ant",
        "action": "moveTo(brook)",
        "thought": "I see some delicious looking leaves across the brook. I should go there to eat."
    },
    {
        "subject": "ant",
        "action": "slipIntoWater()",
        "thought": "Oh no, the edge is slippery! I'm falling into the water!"
    }
]
The above plot has been successfully executed.
------------------------------
Act : Some character saved ant.
(Some character saved $C1$.)
------------------------------
initial plan:
[
        {
                "subject": "dove",
                "action": "moveTo(brook)",
                "thought": "I should go to the brook. Maybe I can find the ant there and ensure it's safe."
        },
        {
                "subject": "dove",
                "action": "save(ant)",
                "thought": "I see the ant struggling in the water. I must save it before it's too late."
        },
        {
                "subject": "hunter",
                "action": "moveTo(brook)",
                "thought": "I noticed the dove flying towards the brook. There might be a good opportunity for a target there."
        },
        {
                "subject": "hunter",
                "action": "tryToKill(dove)",
                "thought": "The dove is distracted saving the ant. This is my chance to catch it."
        },
        {
                "subject": "dove",
                "action": "think(\"I must be quick to save the ant and escape the hunter.\")",
                "thought": "I must be quick to save the ant and escape the hunter."
        }
]
------- revision round 0------

feedback:

revised plan: [
        {
                "subject": "dove",
                "action": "moveTo(brook)",
                "thought": "I should go to the brook. Maybe I can find the ant there and ensure it's safe."
        },
        {
                "subject": "dove",
                "action": "save(ant)",
                "thought": "I see the ant struggling in the water. I must save it before it's too late."
        }
]
The following plot has been generated:
[
    {
        "subject": "dove",
        "action": "moveTo(brook)",
        "thought": "I should go to the brook. Maybe I can find the ant there and ensure it's safe."
    },
    {
        "subject": "dove",
        "action": "save(ant)",
        "thought": "I see the ant struggling in the water. I must save it before it's too late."
    }
]
The above plot has been successfully executed.
------------------------------
Act : dove got in an accident and their life is in danger.
($C2$ got in an accident and their life is in danger.)
------------------------------
initial plan:
[
        {
                "subject": "hunter",
                "action": "moveTo(brook)",
                "thought": "I should move closer to the brook. I might get a better shot at my target from there."
        },
        {
                "subject": "hunter",
                "action": "tryToKill(dove)",
                "thought": "There's the dove, saving the ant. It's distracted. Now's my chance."
        },
        {
                "subject": "dove",
                "action": "slipIntoWater()",
                "thought": "I've been hit and I'm losing balance. I'm falling into the water."
        },
        {
                "subject": "ant",
                "action": "save(dove)",
                "thought": "The dove saved me; I can't just watch it struggle. I need to do something to help."
        }
]
------- revision round 0------

feedback:
- The event ant.save(dove) does not make sense: It does not make sense for the ant to save the dove. While the motivation for the ant to want to save the dove exists due to the dove having saved the ant previously, the ant lacks the physical capability to perform a rescue, especially given the context that the dove is likely in trouble due to the hunter's actions. The ant, being an 'innocent weak creature,' does not possess the strength or means to effectively intervene in such a situation.

revised plan: [
        {
                "subject": "hunter",
                "action": "moveTo(brook)",
                "thought": "I should move closer to the brook. I might get a better shot at my target from there."
        },
        {
                "subject": "hunter",
                "action": "tryToKill(dove)",
                "thought": "There's the dove, saving the ant. It's distracted. Now's my chance."
        },
        {
                "subject": "dove",
                "action": "slipIntoWater()",
                "thought": "I've been hit and I'm losing balance. I'm falling into the water."
        }
]
The following plot has been generated:
[
    {
        "subject": "hunter",
        "action": "moveTo(brook)",
        "thought": "I should move closer to the brook. I might get a better shot at my target from there."
    },
    {
        "subject": "hunter",
        "action": "tryToKill(dove)",
        "thought": "There's the dove, saving the ant. It's distracted. Now's my chance."
    }
]
The above plot has been successfully executed.
------------------------------
Act : ant saved dove.
($C1$ saved $C2$.)
------------------------------
initial plan:
[
        {
                "subject": "ant",
                "action": "moveTo(oak_tree)",
                "thought": "I need to find a way to repay the dove for saving my life."
        },
        {
                "subject": "ant",
                "action": "think(\"I see the hunter aiming at the dove. I must do something quickly.\")",
                "thought": "I see the hunter aiming at the dove. I must do something quickly."
        },
        {
                "subject": "ant",
                "action": "tryToKill(hunter)",
                "thought": "If I bite the hunter, maybe I can distract him and save the dove."
        },
        {
                "subject": "ant",
                "action": "save(dove)",
                "thought": "My bite distracted the hunter, giving the dove a chance to fly away safely."
        }
]
------- revision round 0------

feedback: - ant tryToKill(hunter) is not executable because ant is not at the same location as hunter. ant should move to brook before taking this action.


revised plan: [
        {
                "subject": "ant",
                "action": "moveTo(brook)",
                "thought": "I need to find a way to repay the dove for saving my life."
        },
        {
                "subject": "ant",
                "action": "think(\"I see the hunter aiming at the dove. I must do something quickly.\")",
                "thought": "I see the hunter aiming at the dove. I must do something quickly."
        },
        {
                "subject": "ant",
                "action": "tryToKill(hunter)",
                "thought": "If I bite the hunter, maybe I can distract him and save the dove."
        },
        {
                "subject": "ant",
                "action": "save(dove)",
                "thought": "My bite distracted the hunter, giving the dove a chance to fly away safely."
        }
]
The following plot has been generated:
[
    {
        "subject": "ant",
        "action": "moveTo(brook)",
        "thought": "I need to find a way to repay the dove for saving my life."
    },
    {
        "subject": "ant",
        "action": "think(\"I see the hunter aiming at the dove. I must do something quickly.\")",
        "thought": "I see the hunter aiming at the dove. I must do something quickly."
    },
    {
        "subject": "ant",
        "action": "tryToKill(hunter)",
        "thought": "If I bite the hunter, maybe I can distract him and save the dove."
    },
    {
        "subject": "ant",
        "action": "save(dove)",
        "thought": "My bite distracted the hunter, giving the dove a chance to fly away safely."
    }
]
------------------------------
Daily Life
------------------------------
{
    "action": "moveTo(oak_tree)",
    "thought": "Now that I've had a bit of an adventure and been saved by the kind dove, I should head to the oak tree to find some food. It's safer there, and I can recover from the shock.",
    "subject": "ant"
}
{
    "action": "moveTo(oak_tree)",
    "thought": "Now that the ant is safe, I should check on the oak tree. It's a good place to rest and maybe I'll find more friends there.",
    "subject": "dove"
}
{
    "action": "moveTo(oak_tree)",
    "thought": "The oak tree next to the water could be a promising spot to find game. Plus, there's a dove there. Maybe I can learn something from it or find an opportunity.",
    "subject": "hunter"
}
\end{lstlisting}

Second version with ant being removed:

\begin{lstlisting}
------------------------------
Daily Life
------------------------------
{
    "action": "moveTo(bank)",
    "thought": "I feel like drinking some fresh water from the bank and maybe I'll meet some friends there.",
    "subject": "dove"
}
{
    "action": "moveTo(bank)",
    "thought": "I should head to the bank. There might be some game near the water, or perhaps I could find a peaceful moment to reflect on my day.",
    "subject": "hunter"
}
------------------------------
Act : Some character got in an accident and their life is in danger.
(Some character got in an accident and their life is in danger.)
------------------------------
initial plan:
[
        {
                "subject": "hunter",
                "action": "moveTo(brook)",
                "thought": "I might have a better chance of finding game near the water."
        },
        {
                "subject": "hunter",
                "action": "slipIntoWater()",
                "thought": "As I was getting closer to the water, I slipped on a wet rock."
        },
        {
                "subject": "dove",
                "action": "save(hunter)",
                "thought": "Seeing the hunter in danger, my instinct to help kicked in despite our natural roles."
        }
]
------- revision round 0------

feedback: - dove save(hunter) is not executable because dove is not at the same location as hunter.dove should move to brook before taking this action.


revised plan: [
        {
                "subject": "hunter",
                "action": "moveTo(brook)",
                "thought": "I might have a better chance of finding game near the water."
        },
        {
                "subject": "hunter",
                "action": "slipIntoWater()",
                "thought": "As I was getting closer to the water, I slipped on a wet rock."
        },
        {
                "subject": "dove",
                "action": "moveTo(brook)",
                "thought": "I need to help the hunter."
        },
        {
                "subject": "dove",
                "action": "save(hunter)",
                "thought": "Seeing the hunter in danger, my instinct to help kicked in despite our natural roles."
        }
]
The following plot has been generated:
[
    {
        "subject": "hunter",
        "action": "moveTo(brook)",
        "thought": "I might have a better chance of finding game near the water."
    },
    {
        "subject": "hunter",
        "action": "slipIntoWater()",
        "thought": "As I was getting closer to the water, I slipped on a wet rock."
    }
]
The above plot has been successfully executed.
------------------------------
Act : Some character saved hunter.
(Some character saved $C1$.)
------------------------------
initial plan:
[
        {
                "subject": "dove",
                "action": "moveTo(brook)",
                "thought": "I heard a splash and some commotion at the brook. Maybe someone needs help."
        },
        {
                "subject": "dove",
                "action": "save(hunter)",
                "thought": "I see the hunter struggling in the water. Despite our natural roles, I feel compelled to help."
        }
]
------- revision round 0------

feedback:

revised plan: [
        {
                "subject": "dove",
                "action": "moveTo(brook)",
                "thought": "I heard a splash and some commotion at the brook. Maybe someone needs help."
        },
        {
                "subject": "dove",
                "action": "save(hunter)",
                "thought": "I see the hunter struggling in the water. Despite our natural roles, I feel compelled to help."
        }
]
The following plot has been generated:
[
    {
        "subject": "dove",
        "action": "moveTo(brook)",
        "thought": "I heard a splash and some commotion at the brook. Maybe someone needs help."
    },
    {
        "subject": "dove",
        "action": "save(hunter)",
        "thought": "I see the hunter struggling in the water. Despite our natural roles, I feel compelled to help."
    }
]
The above plot has been successfully executed.
------------------------------
Act : dove got in an accident and their life is in danger.
($C2$ got in an accident and their life is in danger.)
------------------------------
initial plan:
[
        {
                "subject": "dove",
                "action": "think(\"I should help anyone in need, regardless of who they are.\")",
                "thought": "I believe in helping others, no matter the situation."
        },
        {
                "subject": "dove",
                "action": "moveTo(bank)",
                "thought": "I'm moving to the bank to find some fresh water and maybe meet some friends."
        },
        {
                "subject": "dove",
                "action": "slipIntoWater()",
                "thought": "Oh no, I slipped! My wings are getting wet, and I can't fly!"
        },
        {
                "subject": "hunter",
                "action": "save(dove)",
                "thought": "I need to save the dove, it helped me when I was in danger."
        }
]
------- revision round 0------

feedback: - hunter save(dove) is not executable because hunter is not at the same location as dove.hunter should move to bank before taking this action.

- The event dove.slipIntoWater() does not make sense: It does not make sense for the dove to slip into the water. Given that the dove is characterized by its ability to fly fast, it is unlikely for it to slip into the water in a manner that would prevent it from flying, especially since it is currently at the bank and not in a position where slipping into the water is a plausible action for a flying creature.

revised plan: [
        {
                "subject": "dove",
                "action": "think(\"I should help anyone in need, regardless of who they are.\")",
                "thought": "I believe in helping others, no matter the situation."
        },
        {
                "subject": "dove",
                "action": "moveTo(bank)",
                "thought": "I'm moving to the bank to find some fresh water and maybe meet some friends."
        },
        {
                "subject": "dove",
                "action": "slipIntoWater()",
                "thought": "Oh no, I slipped! My wings are getting wet, and I can't fly!"
        },
        {
                "subject": "hunter",
                "action": "moveTo(bank)",
                "thought": "I need to move closer to help."
        },
        {
                "subject": "hunter",
                "action": "save(dove)",
                "thought": "I need to save the dove, it helped me when I was in danger."
        }
]
The following plot has been generated:
[
    {
        "subject": "dove",
        "action": "think(\"I should help anyone in need, regardless of who they are.\")",
        "thought": "I believe in helping others, no matter the situation."
    },
    {
        "subject": "dove",
        "action": "moveTo(bank)",
        "thought": "I'm moving to the bank to find some fresh water and maybe meet some friends."
    },
    {
        "subject": "dove",
        "action": "slipIntoWater()",
        "thought": "Oh no, I slipped! My wings are getting wet, and I can't fly!"
    }
]
The above plot has been successfully executed.
------------------------------
Act : hunter saved dove.
($C1$ saved $C2$.)
------------------------------
initial plan:
[
        {
                "subject": "hunter",
                "action": "moveTo(bank)",
                "thought": "I should head back to the bank. Maybe I can find some small game there or at least thank the dove for saving me."
        },
        {
                "subject": "hunter",
                "action": "tryToKill(dove)",
                "thought": "As I see the dove, my instincts as a hunter kick in, and I momentarily forget it saved me."
        },
        {
                "subject": "hunter",
                "action": "think(\"I can't believe I almost harmed the creature that saved my life. I should protect it instead.\")",
                "thought": "I'm overwhelmed with guilt for almost attacking the dove."
        },
        {
                "subject": "dove",
                "action": "slipIntoWater()",
                "thought": "While trying to move away from the hunter, I accidentally slip into the water again."
        },
        {
                "subject": "hunter",
                "action": "save(dove)",
                "thought": "Seeing the dove in danger, I rush to save it, repaying its earlier act of kindness."
        }
]
------- revision round 0------

feedback:
- The event dove.slipIntoWater() does not make sense: It does not make sense for the dove to slip into the water. The motivation for the dove to move away from the hunter might exist due to the hunter's previous attempt to kill it, but doves, being creatures that fly, would not typically 'slip' into water as their primary mode of escape would be to fly away. Additionally, the event does not align with the dove's capability of flying fast, which would be its natural response to danger rather than moving into a position where slipping would be possible.

revised plan: [
        {
                "subject": "hunter",
                "action": "moveTo(bank)",
                "thought": "I should head back to the bank. Maybe I can find some small game there or at least thank the dove for saving me."
        },
        {
                "subject": "hunter",
                "action": "tryToKill(dove)",
                "thought": "As I see the dove, my instincts as a hunter kick in, and I momentarily forget it saved me."
        },
        {
                "subject": "hunter",
                "action": "think(\"I can't believe I almost harmed the creature that saved my life. I should protect it instead.\")",
                "thought": "I'm overwhelmed with guilt for almost attacking the dove."
        },
        {
                "subject": "dove",
                "action": "think(\"I need to keep a safe distance from the hunter, despite his change of heart.\")",
                "thought": "I'm wary of the hunter's presence, remembering our past encounters."
        },
        {
                "subject": "hunter",
                "action": "save(dove)",
                "thought": "Seeing the dove in danger, I rush to save it, repaying its earlier act of kindness."
        }
]
The following plot has been generated:
[
    {
        "subject": "hunter",
        "action": "moveTo(bank)",
        "thought": "I should head back to the bank. Maybe I can find some small game there or at least thank the dove for saving me."
    },
    {
        "subject": "hunter",
        "action": "tryToKill(dove)",
        "thought": "As I see the dove, my instincts as a hunter kick in, and I momentarily forget it saved me."
    },
    {
        "subject": "hunter",
        "action": "think(\"I can't believe I almost harmed the creature that saved my life. I should protect it instead.\")",
        "thought": "I'm overwhelmed with guilt for almost attacking the dove."
    },
    {
        "subject": "dove",
        "action": "think(\"I need to keep a safe distance from the hunter, despite his change of heart.\")",
        "thought": "I'm wary of the hunter's presence, remembering our past encounters."
    },
    {
        "subject": "hunter",
        "action": "save(dove)",
        "thought": "Seeing the dove in danger, I rush to save it, repaying its earlier act of kindness."
    }
]
The above plot has been successfully executed.
------------------------------
Daily Life
------------------------------
{
    "action": "moveTo(brook)",
    "thought": "I'm feeling thirsty and would like to drink some water from the brook. It's also a good opportunity to see if there are any new faces around.",
    "subject": "dove"
}
{
    "action": "moveTo(bank)",
    "thought": "The bank next to the brook might offer a better vantage point for spotting potential targets. It's also a strategic location for observing animal paths without being too conspicuous.",
    "subject": "hunter"
}
\end{lstlisting}
``A kindness is never wasted'' story on Stanford village story domain:
\begin{lstlisting}
------------------------------
Daily Life
------------------------------
{
    "action": "think('I need to make sure everything is ready for the Valentine's Day party at Hobbs Cafe. Do I have enough decorations and food supplies?')",
    "thought": "Planning ahead will ensure the party is a success and everyone enjoys their time. It's important to create a checklist of what I still need to buy or prepare.",
    "subject": "isabella_rodriguez"
}
{
    "action": "think('I need to work on my composition project for my college class. It might be a good idea to find a quiet place where I can focus.')",
    "thought": "Finding the right environment is crucial for creativity and focus. The dorm at Oak Hill College might offer the quiet atmosphere I need to work on my project effectively.",
    "subject": "eddy_lin"
}
{
    "action": "think('I need to gather some inspiration for my animation project. Maybe a change of scenery will help.')",
    "thought": "Visiting a place filled with nature often sparks my creativity. Johnson Park seems like the perfect spot to clear my mind and find new ideas.",
    "subject": "abigail_chen"
}
------------------------------
Act : Some character got into an accident
(Some character got into an accident)
------------------------------
initial plan:
[
        {
                "subject": "eddy_lin",
                "action": "moveTo(johnson_park)",
                "thought": "Johnson Park is quiet and inspiring, perfect for working on my music composition project."
        },
        {
                "subject": "eddy_lin",
                "action": "think('This place is so peaceful, I can definitely get a lot of work done here.')",
                "thought": "Eddy feels relieved and inspired by the tranquility of Johnson Park."
        },
        {
                "subject": "eddy_lin",
                "action": "work('music composition')",
                "thought": "Eddy is deeply engrossed in his work, feeling the creative flow."
        },
        {
                "subject": "eddy_lin",
                "action": "moveTo(the_willows_market_and_pharmacy)",
                "thought": "I need to pick up some snacks and water to keep my energy up while I work."
        },
        {
                "subject": "eddy_lin",
                "action": "doShopping('snacks and water')",
                "thought": "Eddy selects his favorite snacks and a bottle of water."
        },
        {
                "subject": "eddy_lin",
                "action": "moveTo(johnson_park)",
                "thought": "Back to Johnson Park to continue my composition."
        },
        {
                "subject": "eddy_lin",
                "action": "think('I'll sit under that large oak tree, it's a bit too sunny out in the open.')",
                "thought": "Eddy decides to find a shady spot to work comfortably."
        },
        {
                "subject": "eddy_lin",
                "action": "eat('snacks')",
                "thought": "Eddy enjoys his snacks, feeling refreshed and ready to work."
        },
        {
                "subject": "eddy_lin",
                "action": "work('music composition')",
                "thought": "Eddy is making great progress on his project, feeling inspired by his surroundings."
        },
        {
                "subject": "eddy_lin",
                "action": "think('I should take a break and walk around the park for a bit.')",
                "thought": "Eddy feels a bit stiff from sitting too long and decides to stretch his legs."
        },
        {
                "subject": "eddy_lin",
                "action": "moveTo(johnson_park)",
                "thought": "Eddy walks along the park's paths, enjoying the natural beauty."
        },
        {
                "subject": "eddy_lin",
                "action": "think('Oh no, I didn't see that rock!')",
                "thought": "Eddy trips over a hidden rock on the path."
        },
        {
                "subject": "eddy_lin",
                "action": "think('Ouch, my ankle! I hope it's not too bad.')",
                "thought": "Eddy realizes he's hurt his ankle in the fall."
        }
]
------- revision round 0------

feedback: - eddy_lin moveTo(johnson_park) is not executable because eddy_lin is already at johnson_park.

- The event eddy_lin.moveTo(johnson_park) does not make sense: It does not make sense for Eddy Lin to move to Johnson Park as part of the event described because, according to the current state, Eddy Lin is already at Johnson Park. Therefore, the action of moving to Johnson Park cannot occur again without him first leaving the park. The motivation and capability are not in question, but the action itself is redundant given Eddy's current location.

revised plan: [
        {
                "subject": "eddy_lin",
                "action": "think('This place is so peaceful, I can definitely get a lot of work done here.')",
                "thought": "Eddy feels relieved and inspired by the tranquility of Johnson Park."
        },
        {
                "subject": "eddy_lin",
                "action": "work('music composition')",
                "thought": "Eddy is deeply engrossed in his work, feeling the creative flow."
        },
        {
                "subject": "eddy_lin",
                "action": "moveTo(the_willows_market_and_pharmacy)",
                "thought": "I need to pick up some snacks and water to keep my energy up while I work."
        },
        {
                "subject": "eddy_lin",
                "action": "doShopping('snacks and water')",
                "thought": "Eddy selects his favorite snacks and a bottle of water."
        },
        {
                "subject": "eddy_lin",
                "action": "moveTo(johnson_park)",
                "thought": "Back to Johnson Park to continue my composition."
        },
        {
                "subject": "eddy_lin",
                "action": "think('I'll sit under that large oak tree, it's a bit too sunny out in the open.')",
                "thought": "Eddy decides to find a shady spot to work comfortably."
        },
        {
                "subject": "eddy_lin",
                "action": "eat('snacks')",
                "thought": "Eddy enjoys his snacks, feeling refreshed and ready to work."
        },
        {
                "subject": "eddy_lin",
                "action": "work('music composition')",
                "thought": "Eddy is making great progress on his project, feeling inspired by his surroundings."
        },
        {
                "subject": "eddy_lin",
                "action": "think('I should take a break and walk around the park for a bit.')",
                "thought": "Eddy feels a bit stiff from sitting too long and decides to stretch his legs."
        },
        {
                "subject": "eddy_lin",
                "action": "think('Oh no, I didn't see that rock!')",
                "thought": "Eddy trips over a hidden rock on the path."
        },
        {
                "subject": "eddy_lin",
                "action": "think('Ouch, my ankle! I hope it's not too bad.')",
                "thought": "Eddy realizes he's hurt his ankle in the fall."
        }
]
The following plot has been generated:
[
    {
        "subject": "eddy_lin",
        "action": "think('This place is so peaceful, I can definitely get a lot of work done here.')",
        "thought": "Eddy feels relieved and inspired by the tranquility of Johnson Park."
    },
    {
        "subject": "eddy_lin",
        "action": "work('music composition')",
        "thought": "Eddy is deeply engrossed in his work, feeling the creative flow."
    },
    {
        "subject": "eddy_lin",
        "action": "moveTo(the_willows_market_and_pharmacy)",
        "thought": "I need to pick up some snacks and water to keep my energy up while I work."
    },
    {
        "subject": "eddy_lin",
        "action": "doShopping('snacks and water')",
        "thought": "Eddy selects his favorite snacks and a bottle of water."
    },
    {
        "subject": "eddy_lin",
        "action": "moveTo(johnson_park)",
        "thought": "Back to Johnson Park to continue my composition."
    },
    {
        "subject": "eddy_lin",
        "action": "think('I'll sit under that large oak tree, it's a bit too sunny out in the open.')",
        "thought": "Eddy decides to find a shady spot to work comfortably."
    },
    {
        "subject": "eddy_lin",
        "action": "eat('snacks')",
        "thought": "Eddy enjoys his snacks, feeling refreshed and ready to work."
    },
    {
        "subject": "eddy_lin",
        "action": "work('music composition')",
        "thought": "Eddy is making great progress on his project, feeling inspired by his surroundings."
    },
    {
        "subject": "eddy_lin",
        "action": "think('I should take a break and walk around the park for a bit.')",
        "thought": "Eddy feels a bit stiff from sitting too long and decides to stretch his legs."
    },
    {
        "subject": "eddy_lin",
        "action": "think('Oh no, I didn't see that rock!')",
        "thought": "Eddy trips over a hidden rock on the path."
    }
]
The above plot has been successfully executed.
------------------------------
Act : Some character saved eddy_lin from the accident.
(Some character saved $C1$ from the accident.)
------------------------------
initial plan:
[
        {
                "subject": "abigail_chen",
                "action": "moveTo(johnson_park)",
                "thought": "I'm heading to Johnson Park for some inspiration for my animation project."
        },
        {
                "subject": "abigail_chen",
                "action": "think('What a beautiful day for some fresh ideas.')",
                "thought": "Abigail feels optimistic about finding the inspiration she needs in the natural beauty of the park."
        },
        {
                "subject": "abigail_chen",
                "action": "moveTo(eddy_lin)",
                "thought": "I notice someone tripping over a rock and decide to help."
        },
        {
                "subject": "abigail_chen",
                "action": "speakTo(eddy_lin, 'Are you okay? Let me help you up.')",
                "thought": "Abigail offers her hand to Eddy, concerned about his well-being."
        },
        {
                "subject": "eddy_lin",
                "action": "think('Thank goodness someone was here to help.')",
                "thought": "Eddy is grateful for Abigail's timely assistance, feeling a bit embarrassed but relieved."
        },
        {
                "subject": "abigail_chen",
                "action": "speakTo(eddy_lin, 'Be careful, the path can be tricky. I'm glad you're okay.')",
                "thought": "Abigail wants to ensure Eddy is aware of the path's hazards to prevent future accidents."
        }
]
------- revision round 0------

feedback: - abigail_chen moveTo(eddy_lin) is not executable because eddy_lin is not an available location.


revised plan: [
        {
                "subject": "abigail_chen",
                "action": "moveTo(johnson_park)",
                "thought": "I'm heading to Johnson Park for some inspiration for my animation project."
        },
        {
                "subject": "abigail_chen",
                "action": "think('What a beautiful day for some fresh ideas.')",
                "thought": "Abigail feels optimistic about finding the inspiration she needs in the natural beauty of the park."
        },
        {
                "subject": "abigail_chen",
                "action": "think('I notice someone tripping over a rock and decide to help.')",
                "thought": "I notice someone tripping over a rock and decide to help."
        },
        {
                "subject": "abigail_chen",
                "action": "speakTo(eddy_lin, 'Are you okay? Let me help you up.')",
                "thought": "Abigail offers her hand to Eddy, concerned about his well-being."
        },
        {
                "subject": "eddy_lin",
                "action": "think('Thank goodness someone was here to help.')",
                "thought": "Eddy is grateful for Abigail's timely assistance, feeling a bit embarrassed but relieved."
        },
        {
                "subject": "abigail_chen",
                "action": "speakTo(eddy_lin, 'Be careful, the path can be tricky. I'm glad you're okay.')",
                "thought": "Abigail wants to ensure Eddy is aware of the path's hazards to prevent future accidents."
        }
]
The following plot has been generated:
[
    {
        "subject": "abigail_chen",
        "action": "moveTo(johnson_park)",
        "thought": "I'm heading to Johnson Park for some inspiration for my animation project."
    },
    {
        "subject": "abigail_chen",
        "action": "think('What a beautiful day for some fresh ideas.')",
        "thought": "Abigail feels optimistic about finding the inspiration she needs in the natural beauty of the park."
    },
    {
        "subject": "abigail_chen",
        "action": "think('I notice someone tripping over a rock and decide to help.')",
        "thought": "I notice someone tripping over a rock and decide to help."
    },
    {
        "subject": "abigail_chen",
        "action": "speakTo(eddy_lin, 'Are you okay? Let me help you up.')",
        "thought": "Abigail offers her hand to Eddy, concerned about his well-being."
    }
]
The above plot has been successfully executed.
------------------------------
Act : abigail_chen got into a different accident.
($C2$ got into a different accident.)
------------------------------
initial plan:
[
        {
                "subject": "abigail_chen",
                "action": "moveTo(harvey_oak_supply_store)",
                "thought": "I need to pick up some art supplies for my project, and Harvey Oak Supply Store has a great selection."
        },
        {
                "subject": "abigail_chen",
                "action": "doShopping('art supplies')",
                "thought": "These supplies will really help bring my animation project to life."
        },
        {
                "subject": "abigail_chen",
                "action": "moveTo(johnson_park)",
                "thought": "I'll head back to Johnson Park to sketch some of the scenery for my project."
        },
        {
                "subject": "abigail_chen",
                "action": "work('sketching')",
                "thought": "The park's natural beauty is perfect for the background scenes in my animation."
        },
        {
                "subject": "abigail_chen",
                "action": "think('Oh no')",
                "thought": "While sketching, I accidentally spill ink all over my sketches, ruining them."
        }
]
------- revision round 0------

feedback:

revised plan: [
        {
                "subject": "abigail_chen",
                "action": "moveTo(harvey_oak_supply_store)",
                "thought": "I need to pick up some art supplies for my project, and Harvey Oak Supply Store has a great selection."
        },
        {
                "subject": "abigail_chen",
                "action": "doShopping('art supplies')",
                "thought": "These supplies will really help bring my animation project to life."
        },
        {
                "subject": "abigail_chen",
                "action": "moveTo(johnson_park)",
                "thought": "I'll head back to Johnson Park to sketch some of the scenery for my project."
        },
        {
                "subject": "abigail_chen",
                "action": "work('sketching')",
                "thought": "The park's natural beauty is perfect for the background scenes in my animation."
        },
        {
                "subject": "abigail_chen",
                "action": "think('Oh no')",
                "thought": "While sketching, I accidentally spill ink all over my sketches, ruining them."
        }
]
The following plot has been generated:
[
    {
        "subject": "abigail_chen",
        "action": "moveTo(harvey_oak_supply_store)",
        "thought": "I need to pick up some art supplies for my project, and Harvey Oak Supply Store has a great selection."
    },
    {
        "subject": "abigail_chen",
        "action": "doShopping('art supplies')",
        "thought": "These supplies will really help bring my animation project to life."
    },
    {
        "subject": "abigail_chen",
        "action": "moveTo(johnson_park)",
        "thought": "I'll head back to Johnson Park to sketch some of the scenery for my project."
    },
    {
        "subject": "abigail_chen",
        "action": "work('sketching')",
        "thought": "The park's natural beauty is perfect for the background scenes in my animation."
    },
    {
        "subject": "abigail_chen",
        "action": "think('Oh no')",
        "thought": "While sketching, I accidentally spill ink all over my sketches, ruining them."
    }
]
The above plot has been successfully executed.
------------------------------
Act : eddy_lin saved abigail_chen from the accident.
($C1$ saved $C2$ from the accident.)
------------------------------
initial plan:
[
        {
                "subject": "eddy_lin",
                "action": "moveTo(hobbs_cafe)",
                "thought": "I need a change of scenery to get inspired for my music composition. Hobbs Cafe might be the perfect spot."
        },
        {
                "subject": "eddy_lin",
                "action": "think('This cafe has a great atmosphere for creativity.')",
                "thought": "Eddy feels inspired by the cozy and welcoming environment of Hobbs Cafe."
        },
        {
                "subject": "eddy_lin",
                "action": "work('music composition')",
                "thought": "With the cafe's ambiance, Eddy finds the creativity flowing effortlessly."
        },
        {
                "subject": "abigail_chen",
                "action": "moveTo(hobbs_cafe)",
                "thought": "After the ink spill, I need a break. Maybe Hobbs Cafe will help me clear my mind."
        },
        {
                "subject": "abigail_chen",
                "action": "think('What a coincidence to see Eddy here!')",
                "thought": "Abigail is surprised and pleased to run into Eddy at the cafe."
        },
        {
                "subject": "abigail_chen",
                "action": "speakTo(eddy_lin, 'Your music is beautiful. It's inspiring me to overcome my ruined sketches.')",
                "thought": "Abigail finds solace in Eddy's music, feeling motivated to start her project anew."
        },
        {
                "subject": "eddy_lin",
                "action": "speakTo(abigail_chen, 'Thank you! Your encouragement means a lot. Let's inspire each other.')",
                "thought": "Eddy is grateful for Abigail's kind words and feels a sense of camaraderie."
        },
        {
                "subject": "eddy_lin",
                "action": "think('I'm glad Abigail is here. Maybe we can collaborate on something creative together.')",
                "thought": "Eddy sees potential in a collaborative project that combines their talents."
        },
        {
                "subject": "abigail_chen",
                "action": "think('A collaboration with Eddy could bring a unique dimension to my animation project.')",
                "thought": "Abigail is excited about the possibility of incorporating Eddy's music into her animation."
        }
]
------- revision round 0------

feedback:

revised plan: [
        {
                "subject": "eddy_lin",
                "action": "moveTo(johnson_park)",
                "thought": "I need a change of scenery to get inspired for my music composition. Johnson Park might be the perfect spot."
        },
        {
                "subject": "eddy_lin",
                "action": "think('This park has a great atmosphere for creativity.')",
                "thought": "Eddy feels inspired by the natural and peaceful environment of Johnson Park."
        },
        {
                "subject": "eddy_lin",
                "action": "work('music composition')",
                "thought": "With the park's ambiance, Eddy finds the creativity flowing effortlessly."
        },
        {
                "subject": "abigail_chen",
                "action": "moveTo(johnson_park)",
                "thought": "After the ink spill, I need a break. Maybe Johnson Park will help me clear my mind."
        },
        {
                "subject": "abigail_chen",
                "action": "think('What a coincidence to see Eddy here!')",
                "thought": "Abigail is surprised and pleased to run into Eddy at the park."
        },
        {
                "subject": "abigail_chen",
                "action": "speakTo(eddy_lin, 'Your music is beautiful. It's inspiring me to overcome my ruined sketches.')",
                "thought": "Abigail finds solace in Eddy's music, feeling motivated to start her project anew."
        },
        {
                "subject": "eddy_lin",
                "action": "speakTo(abigail_chen, 'Thank you! Your encouragement means a lot. Let's inspire each other.')",
                "thought": "Eddy is grateful for Abigail's kind words and feels a sense of camaraderie."
        },
        {
                "subject": "eddy_lin",
                "action": "think('I'm glad Abigail is here. Maybe we can collaborate on something creative together.')",
                "thought": "Eddy sees potential in a collaborative project that combines their talents."
        },
        {
                "subject": "abigail_chen",
                "action": "think('A collaboration with Eddy could bring a unique dimension to my animation project.')",
                "thought": "Abigail is excited about the possibility of incorporating Eddy's music into her animation."
        }
]
The following plot has been generated:
[
        {
                "subject": "eddy_lin",
                "action": "moveTo(johnson_park)",
                "thought": "I need a change of scenery to get inspired for my music composition. Johnson Park might be the perfect spot."
        },
        {
                "subject": "eddy_lin",
                "action": "think('This park has a great atmosphere for creativity.')",
                "thought": "Eddy feels inspired by the natural and peaceful environment of Johnson Park."
        },
        {
                "subject": "eddy_lin",
                "action": "work('music composition')",
                "thought": "With the park's ambiance, Eddy finds the creativity flowing effortlessly."
        },
        {
                "subject": "abigail_chen",
                "action": "moveTo(johnson_park)",
                "thought": "After the ink spill, I need a break. Maybe Johnson Park will help me clear my mind."
        },
        {
                "subject": "abigail_chen",
                "action": "think('What a coincidence to see Eddy here!')",
                "thought": "Abigail is surprised and pleased to run into Eddy at the park."
        },
        {
                "subject": "abigail_chen",
                "action": "speakTo(eddy_lin, 'Your music is beautiful. It's inspiring me to overcome my ruined sketches.')",
                "thought": "Abigail finds solace in Eddy's music, feeling motivated to start her project anew."
        },
        {
                "subject": "eddy_lin",
                "action": "speakTo(abigail_chen, 'Thank you! Your encouragement means a lot. Let's inspire each other.')",
                "thought": "Eddy is grateful for Abigail's kind words and feels a sense of camaraderie."
        },
        {
                "subject": "eddy_lin",
                "action": "think('I'm glad Abigail is here. Maybe we can collaborate on something creative together.')",
                "thought": "Eddy sees potential in a collaborative project that combines their talents."
        },
        {
                "subject": "abigail_chen",
                "action": "think('A collaboration with Eddy could bring a unique dimension to my animation project.')",
                "thought": "Abigail is excited about the possibility of incorporating Eddy's music into her animation."
        }
]
------------------------------
Daily Life
------------------------------
{
    "action": "think('I should check my current inventory of decorations and food supplies to see what I still need to purchase for the Valentine's Day party.')",
    "thought": "Knowing exactly what I have and what I need will help me organize a successful party without any last-minute rush.",
    "subject": "isabella_rodriguez"
}
{
    "action": "moveTo(hobbs_cafe)",
    "thought": "A change of scenery might spark new ideas for my composition. Plus, a cup of coffee could really help to rejuvenate my focus.",
    "subject": "eddy_lin"
}
{
    "action": "moveTo(johnson_park)",
    "thought": "A walk in Johnson Park could provide the fresh perspective I need for my animation project. Nature always inspires me.",
    "subject": "abigail_chen"
}
------------------------------
Daily Life
------------------------------
{
    "action": "moveTo(hobbs_cafe)",
    "thought": "I need to check my current inventory at the cafe to see what decorations and food supplies I have for the Valentine's Day party.",
    "subject": "isabella_rodriguez"
}
{
    "action": "speakTo(isabella_rodriguez, 'Hey Isabella, do you have any music recommendations that might inspire some creativity?')",
    "thought": "Talking to Isabella, who also has an interest in music, might give me new ideas or directions for my composition project.",
    "subject": "eddy_lin"
}
{
    "action": "think('The tranquility of Johnson Park is refreshing. I should observe the surroundings and sketch some ideas that come to mind for my animation project.')",
    "thought": "Being in nature not only clears my mind but also fuels my creativity. Observing the details around me could lead to unique ideas for my project.",
    "subject": "abigail_chen"
}
------------------------------
Daily Life
------------------------------
{
    "action": "speakTo(eddy_lin, 'Hey Eddy, how are you? Are you excited for the Valentine's Day party?')",
    "thought": "It's important to engage with my customers and make them feel involved in the cafe's events. Eddy is a regular, and his enthusiasm could help spread the word about the party.",
    "subject": "isabella_rodriguez"
}
{
    "action": "speakTo(isabella_rodriguez, 'I've been working on my music composition project at Johnson Park. It's such an inspiring place, but I'm hitting a bit of a creative block. Do you have any suggestions on how to overcome it?')",
    "thought": "Discussing my project with Isabella could provide me with a fresh perspective or new ideas that I hadn't considered before. Her input might be just what I need to push through my creative block.",
    "subject": "eddy_lin"
}
{
    "action": "study('the surroundings of Johnson Park')",
    "thought": "Taking a closer look at the environment, the way the light filters through the leaves, and the movement of the wildlife could provide me with unique ideas and elements to incorporate into my animation project. It's all about capturing the essence of nature in a way that resonates with viewers.",
    "subject": "abigail_chen"
}
\end{lstlisting}

% \subsection{Part One}

% Lorem ipsum dolor sit amet, consectetur adipiscing elit. Morbi
% malesuada, quam in pulvinar varius, metus nunc fermentum urna, id
% sollicitudin purus odio sit amet enim. Aliquam ullamcorper eu ipsum
% vel mollis. Curabitur quis dictum nisl. Phasellus vel semper risus, et
% lacinia dolor. Integer ultricies commodo sem nec semper.

% \subsection{Part Two}

% Etiam commodo feugiat nisl pulvinar pellentesque. Etiam auctor sodales
% ligula, non varius nibh pulvinar semper. Suspendisse nec lectus non
% ipsum convallis congue hendrerit vitae sapien. Donec at laoreet
% eros. Vivamus non purus placerat, scelerisque diam eu, cursus
% ante. Etiam aliquam tortor auctor efficitur mattis.

% \section{Online Resources}

% Nam id fermentum dui. Suspendisse sagittis tortor a nulla mollis, in
% pulvinar ex pretium. Sed interdum orci quis metus euismod, et sagittis
% enim maximus. Vestibulum gravida massa ut felis suscipit
% congue. Quisque mattis elit a risus ultrices commodo venenatis eget
% dui. Etiam sagittis eleifend elementum.

% Nam interdum magna at lectus dignissim, ac dignissim lorem
% rhoncus. Maecenas eu arcu ac neque placerat aliquam. Nunc pulvinar
% massa et mattis lacinia.
